# Supplementary material for: Statistical and computational thresholds for the planted $k$-densest sub-hypergraph problem
Source: arXiv:2011.11500 source file (2021-01-28)
Supplement: Supplementary file 1 [file appendix_postponed_proofs.tex]

\subsection{Probability tools}
We shall use the well-known inequalities on \emph{tail distribution of Gaussians}: For any $X \sim \Gaussian(\mu,\sigma^2)$ and any $c>0$, it holds that (see \cite[Section~7.1]{feller2008introduction})
\begin{equation}
\label{eq:Gaussian}
(\frac{1}{c} - \frac{1}{c^2})\cdot  \frac{e^{-c^2/2\sigma^2}}{\sqrt{2\pi}} \leq \Pr(X > \beta+c) \leq \frac{1}{c}\cdot  \frac{e^{-c^2/2\sigma^2}}{\sqrt{2\pi}} \ .
\end{equation}
We typically deal with solutions (events) which are \emph{dependent}, for which the following \emph{Chung-Erd\"os inequality} and the well-known \emph{union bound} will be used: Given $n$ events $A_1,\ldots A_n$, it holds that (see \cite{szpankowski2011average})
\begin{align}
\frac{\left(\sumP\right)^2}{\sumP + \sumPdep} \leq \sumPunion \label{eq:cebound}\\
\leq \sumP \label{eq:union-bound}
\end{align}
where the first inequality is the \emph{Chung-Erd\"os} bound and the second one is the \emph{union bound}.

\subsection{Proof of \texorpdfstring{\Cref{th:UB}}{}}
Throughout this section, we shall identify a solution simply by its total weight $S$ as defined in  \cref{eq:weight-def}. With slight abuse of notation we denote by `$\S_m$' suitable (sub)sets of solutions and write $S\in \S_m$ to denote the weight $S$ of a particular in that set, when this is clear from the context. The weight of the planted solution is $\plant$. Finally, for any set $\S$, $\max(\S) \equiv \max_{S \in \S} x$.

\bigskip

To study the recoverability thresholds we analyze the behaviour of the maximum likelihood estimator of the planted solution $K_{planted}$, that it can be easily identified as the $k$-densest sub-hypergraph (see Theorem 4 in \cite{corinzia2019} for a proof). We consider the generic $k'+1$-partial recover for the MLE estimator. Exact recovery corresponds to the case $k'=k-1$. %In the following, most proofs are omitted and reported in the long version of the paper.
\begin{lemma}
	Let $\recover^{(k')}$ be the probability that the MLE recovers more than $k'$ nodes from the planted solution, and $\fail^{(k')}=1-\recover^{(k')}$ the probability that it fails in doing so. 
	For any $m$ let $\S_m$ denote the set of all solutions that share exactly $m$ nodes with the planted solution $\plant$.  Then the following holds:
	\begin{align}
	&\fail^{(k')} \leq \sum_{m=0}^{k'}\Pr\left(\plant\leq \max(\S_{m})\right)\ && \label{eq:UB:max-based} \\
	&\fail \equiv \fail^{(k-1)} \geq  \Pr(\plant < \max(\S_{k'})) 
	\label{eq:LB:max-based}
	\end{align}
	for any $k' \in\{0,\ldots,k-1\}$.
\end{lemma}
\begin{proof}
	The upper bound in \eqref{eq:UB:max-based} follows since $\plant>S$ for all $S \in \S_0\cup \S_1\cup \cdots \cup \S_{m}$. Then the MLE must return $\plant$ or some solution in $\S_{m+1} \cup \cdots \cup \S_k$, and the inequality follow from the union bound on the probability $\Pr\left(\bigcup_{m=0}^{k'} \left\{\plant\leq \max(\S_{m})\right\}\right)$. For the lower bound in \eqref{eq:LB:max-based} we can observe that if $\plant< \max(\S_{k'})$ for some $k' <k$, then the MLE cannot return $\plant$, and thus it fails to exactly recover the planted solution.
\end{proof}
Intuitively speaking, our goal is to distinguish between the case in which recovery is possible from the one in which it is impossible, i.e., whether $\gamma$ is in the regime such that
\begin{align*}
\Pr(\fail^{(k')})
\rightarrow 0 && \text{ or } && \Pr(\fail^{(k')}) \rightarrow 1 \ .
\end{align*}
We shall reduce this question to the study of the probabilities $\Pr(\plant < \max(\S_{m}))$,  so to determine the values of $\gamma$ for which 
\begin{align*}
\Pr(\plant\leq \max(\S_{m})) \rightarrow 0 && \text{ or } && \Pr(\plant\leq \max(\S_{m})) \rightarrow 1
\end{align*}
where in the left scenario (recovery possible) we need these probabilities to go to zero \emph{sufficiently fast} to apply the union bound (\cref{eq:UB:max-based}) over all different $m$.

For the purpose of the analysis, we define the following quantities depending on $k' \in \{0,\ldots, k-1\}$:
\begin{align*}
d({k'}) \equiv \binom{k}{h} - \binom{k'}{h} = \binom{k}{h}(1 - \rho(k')), && Q_{k'} \equiv \binom{n-k}{k-{k'}}, \\
M_{k'} \equiv \binom{k}{k'}\binom{n-k}{k-{k'}}=\binom{k}{k-{k'}}\binom{n-k}{k-{k'}}
\end{align*} 
Note that, for each \emph{fixed} subset of $k'$ nodes of the planted solution, there are $Q_{k'}$ solutions that share these $k'$ nodes with the planted solution. Moreover, there are exactly $M_{k'}$ solutions that share $k'$ nodes with the planted solution. Each such solution sharing $k'$ nodes with the planted solution differs in $d(k')$ edges with the planted solution.
Finally, we let
\begin{align}
\label{eq:threshold-plus-min}
t_\Delta \equiv \sqrt{\Delta 2 \log n} \ .
\end{align}
\begin{lemma}
	\label{le:UB-concentration}
	Fix an arbitrary subset $F \subset K_{planted}$ of ${k'}$ nodes of the planted solution, with ${k'}\in \{0,\ldots,k-1\}$,   and let $\S_{k'}^{(F)}$ be the set of all solutions that share exactly this set of ${k'}$ nodes with the planted solution. For any $S\in \S_{k'}^{(F)}$ let $S^{(-F)}$ denote the sum of the weights in the non-common part, that is the sum of $d({k'}) = \binom{k}{h} - \binom{k'}{h}$ edge weights in $S$ and with none of their nodes contained in $F$. Denote by $\S_{k'}^{(-F)}$ the set of all the $S^{(-F)}$. For any $\Delta>0$ and any $S^{(-F)}$ as above, it holds that
	\begin{equation}
	\label{eq:bound-generic:m-intersecting}
	\Pr \left(S^{(-F)}  > t_\Delta \right) \leq p_{{k'},\Delta} \equiv \left(\frac{1}{n}\right)^{\frac{\Delta}{d({k'})}} \frac{1}{\sqrt{2\pi \Delta} \cdot \sqrt{2\log n}} \ .
	\end{equation}
	Moreover, the following holds:
	\begin{align}
	&\Pr\left(\max(\S_{k'}^{(-F)}) >  t_\Delta \right) \leq Q_{k'} \cdot p_{{k'},\Delta}\label{eq:LB-bound:m-intersecting} \\ 
	&\Pr\left(\plant^{(-F)} < d({k'}) \beta - t_\Delta \right) \leq p_{{k'},\Delta} \label{eq:UB-bound:planted}
	\end{align}
	where $\left|\S_{k'}^{(-F)} \right|=\binom{n-k}{k - {k'}} = Q_{k'}$.
\end{lemma}
%\begin{proof}
%Given in %\crefapp{app:proofs_UB}.
%\end{proof}

%\begin{cor}
%		For any $\Delta = \Omega\left(\frac{d(m)}{\log N}\right)$, it holds that $p_{m,\Delta} \rightarrow 0$ and therefore 
%		\begin{align*}
%		\Pr\left(\plant^{(-F)} < d(m) \mu -\sigma \sqrt{\Delta 2\log N} \right) \rightarrow 0 \ .
%		\end{align*}
%\end{cor}

\begin{theorem}
	\label{th:UB-with-eta}
	For every $\eta \geq 0$ and for every ${k'} \in \{0,\ldots, k-1\}$, let 
	$\gamma^{({k'})}_{UB_{\eta}} \equiv  \sqrt{\frac{\binom{k}{h}}{k}}\cdot \sqrt{\frac{1}{d(k')}} \cdot UB_{\eta}({k'}) $
	%$\gamma^{({k'})}_{UB_{\eta}} \equiv  \sqrt{\frac{\binom{k}{h}}{k d({k'})}} \cdot UB_{\eta}({k'}) $ 
	where 
	\begin{align}
	\label{eq:UB:gamma-k}
	UB_{\eta}({k'}) \equiv \sqrt{\frac{\log M_{k'}}{\log n}+\eta}  + \sqrt{\frac{\log \binom{k}{k'}}{\log n}+\eta}  \ .	  
	\end{align}
	Then, for any $\gamma > \gamma^{({k'})}_{UB_{\eta}}$ it holds that
	\[
	\Pr\left(\max(\S_{k'}) >  \plant\right) \in O\left(\frac{\sqrt{\log n}}{n^{\eta}}\right)\ .
	\]
\end{theorem}

\begin{proof}[Proof Idea]
By the union bound over the ${k \choose k'}$ possible fixed subsets $F$ of $k'$ nodes, we get $$
\Pr\left(\max(\S_{k'}) >  \plant\right) \leq   \binom{k}{{k'}} \cdot \Pr(\max(\S_{k'}^{(-F)})> \plant^{(-F)}).$$ 
Moreover, for any $t$, we have
$\Pr\left(\max(\S_{k'}^{(-F)})> \plant^{(-F)}\right) \leq  
\Pr\left(\max(\S_{k'}^{(-F)})>t\right) +  \Pr\left(t\geq  \plant^{(-F)}\right) $. Calculations show that, since $\gamma>\gamma^{({k'})}_{UB_{\eta}}$, there exists a particular $t$ such that \Cref{le:UB-concentration} implies that both these two probabilities go to $0$ sufficiently fast. See \Cref{app:proofs_UB} for the full proof.
\end{proof}
The rates $\rate{k}$ and $\rate{k-k'}$ defined by \cref{eq:rate}
provide upper bounds for the fractions in \cref{eq:UB:gamma-k}. Using the union bound over all $m=\{0,\ldots, k'\}$ we can set $\eta=\beta_0''$ so that the right hand side of  \cref{eq:UB:max-based} goes to $0$. This leads to the upper bound in \Cref{th:UB}.

\subsection{Proof of \Cref{le:cover}}
\begin{proof}
We construct $\cN_r$ by a simple iterative greedy procedure. 
Starting from an arbitrary $x\in \CNK$, include $x$ into $\cN_r$ and remove all solutions in $\CNK$ which intersect $x$ in at least $r$ nodes.  Iterate this step with the remaining solutions in $\CNK$ not considered before. Every time we include one new solution in $\cN_r$, we  remove (at most) $B(r)$  solutions from $\CNK$. So, in total we can collect in $\cN_r$ at least $\lceil|\CNK|/B(r)\rceil = \lceil\binom{n}{k}/B(r) \rceil$ many solutions. This proves part (3). Part (1) holds by construction, and part (2) is because otherwise $x\not \in \cN_r$ would have been included by this procedure.
\end{proof}
	\subsection{Proof of \Cref{le:R-lb}}
	\begin{proof}Since $\binom{k}{d} \leq 2^k$  and $\binom{n-k}{k-d}\leq \binom{n}{k - \share}$, we get the following upper bound
		\begin{align}
		B(r)  \leq 	2^k \binom{n }{k - \share}(k - \share) \ .
		\end{align}
		Therefore
		\begin{align}\label{eq:R:log-diff}
		R(r) =& \log \frac{\binom{n}{k}}{B(r)} \geq \log \binom{n}{k} -\left[ k +\log \binom{n}{k - \share}  + \log (k - \share)\right] \ . 
		\end{align}
		Using standard inequalities on the binomial coefficients,  
		\begin{align}
		\label{eq:log-bonimial}
		a(\log b - \log a) \leq \log {b \choose a} \leq a(1+\log b - \log a)  \ ,
		\end{align}
		we get
		\begin{align}
		\log \binom{n}{k} \geq k(\log n - \log k) = k (1-\alpha)\log n & \label{eq:log-N-k}
		\end{align}	
		and
		\begin{align}
		\log \binom{n}{k - \share}  \leq& (k-\share) (1+\log n - \log (k-\share)) \nonumber \\
		\lesssim & (k-\share) (1 - \alpha)\log n   \ ,
		\label{eq:log-three-binoms}
		\end{align}
		where the last inequality follows from $r \leq \lambda k$ and, in particular, $\log (k - r)\geq \log (k-\lambda k) = \log k + \log(1-\lambda)\approx \log k = \alpha \log n$. Hence
		\begin{align}
		\rate{C(r)}\stackrel{\eqref{eq:rate}}{=}\frac{R(r)}{\log n} \gtrsim  &  k(1-\alpha) - (k -\share) (1 - \alpha) - \frac{k + \log (k-\share)}{\log n} \nonumber \\ 
		= &  \share (1 - \alpha) - o(\share) \approx r(1-\alpha) \ ,  
		\end{align}
		where the last equality is due to $r = \omega(\frac{k}{\log n}) $.
	\end{proof}

\subsection{Proof of \Cref{th:LB:max-Gaussians}}\label{sec:proof:UB}
This proof of this lower bound is based on the following result on tail bounds on the \emph{maximum} of  Gaussians with \emph{bounded}  correlation \cite{lopes2018maximum}.

\begin{lemma}[Theorem~2.2 in \cite{lopes2018maximum}]\label{le:max-Gaussians}
	For any constant $\delta_0 \in (0,1)$, the maximum of  $N$ possibly dependent Gaussian random variables $X_1,\ldots,X_N \sim \Gaussian(0,\sigma_X^2)$ satisfies
	\begin{align}\label{eq:max-Gaussians}
	\Pr\left(\max(X_1,\ldots,X_N) \leq \sigma_X \cdot \delta_0 \sqrt{2(1-\rho_0) \log N}\right) \leq C \cdot \frac{\log^\alpha N}{N^\beta}
	\end{align}
	where  $C=C(\delta_0,\rho_0)$ is a constant depending only on $\delta_0$ and $\rho_0$, 
	\begin{align}\label{eq:max-Gaussians-constants}
	\alpha = \frac{1 - \rho_0}{\rho_0} (1 - \delta_0) \ , && \text{ and } && \beta = \frac{1 - \rho_0}{\rho_0} (1 - \delta_0)^2 \ .
	\end{align}
\end{lemma}

We here outline a road map of the proof: i) analyze conditions for vanishing correlation between solutions ($\rho(r)\rightarrow 0$), ii) 
using \cref{le:max-Gaussians} we show that vanishing correlation implies the concentration of the maximum of a given cover of solutions (via rate the cover rate $\rate{C(r)}$), iii) using a lower bound on the rate of the cover, we provide a respective lower bound of the recovery threshold.
\begin{lemma}[vanishing correlation]\label{le:vanishing-corr} The correlation between any two solutions sharing $\share$ nodes is $\rho=\rho(\share) = \frac{\binom{\share}{h}}{\binom{k}{h}}$ and it vanishes in each of the following two regimes: 
	\begin{enumerate}
		\item For $h=\omega(1)$ and $\share \leq \lambda k$ for any constant $\lambda$ satisfying
		\begin{align}\label{eq:linear-ell-cases}
		\begin{cases}
		\lambda < 1 & \text{ for } h = o(\sqrt{k})
		\\
		\lambda <1/e & \text{ otherwise }
		\end{cases}
		\end{align}
		%\item For $h = \omega(1)$,
		%and for any $\share \leq \frac{k}{c_0}$ for constant $c_0>e$.
		\item For $h = O(1)$ and for any $\share = o(k)$. 
	\end{enumerate}
\end{lemma}

\begin{proof} 
	Observe that,
	\begin{align*}
	k(k-1)\cdots (k-h+1) \geq (k - h)^h = \left(1 - \frac{h}{k}\right)^h k^h \geq \left(1 - \frac{h^2}{k}\right) k^h
	\end{align*}
	and therefore 
	\begin{align*}
	\frac{{\share \choose h}}{{k \choose h}} &= \frac{\share!}{h!(\share-h)!}\frac{h!(k-h)!}{\share !} 
	=\frac{\share(\share-1)\cdots (\share-h+1)}{k(k-1)\cdots (k-h+1)} \leq \left(\frac{\share}{k}\right)^h \frac{1}{\left(1 - \frac{h^2}{k}\right)} \leq 
	\frac{\lambda^h }{\left(1 - \frac{h^2}{k}\right)} \ .
	\end{align*}
	For $h = o(\sqrt{k})$ and $h=\omega(1)$ the latter quantity converges to $0$ for any constant $\lambda<1$.  As for the other case in \eqref{eq:linear-ell-cases}, we have 
	\begin{align*}
	\frac{\binom{\share}{h}}{\binom{k}{h}} & \leq \frac{e^h \share ^h}{h^h} \cdot  \frac{h^h}{k^h} = \left(\frac{e \cdot \share}{k}\right)^h \leq \left(e \lambda \right)^h \rightarrow 0
	\end{align*}
	where the asymptotics follows from $e < c_0$ and $h \rightarrow \infty$. As for the second case, since $h=\Theta(1)$ we have  $\binom{\share}{h} = \Theta(\share^{h})$ and $\binom{k}{h} = \Theta(k^{h})$,  and thus  $\share \ll k$ implies $\binom{\share}{h} \ll \binom{k}{h}$.    
\end{proof}

\begin{lemma}[concentration of the maximum]\label{le:max-concentration}
	For $\share$ such that the correlation $\rho(\share)$ vanishes, i.e, $\rho(\share) \rightarrow 0$, and for any constant $\epsilon_0\in (0,1)$  
	\begin{align}\label{eq:cor-max-concentration}
	\Pr\left(\max(\cN_r) \leq (1- \epsilon_0) \cdot \sigma_k  \sqrt{\rate{C(r)}\cdot 2\log n}\right) \rightarrow 0
	\end{align}
	where $\sigma_k = \sqrt{\binom{k}{h}}$.
	%	For any $\share$ such that the correlation $\rho(\share)$ vanishes and for $MAX(\cN_r) \equiv \max \{S \in \cN_r\}$ and $C(r) = |\cN_r|$ it holds that
	%	\begin{align}\label{eq:max-concentration}
	%	\Pr\left(MAX(\cN_r) \leq (1- \epsilon_0) \cdot \sigma_h  \sqrt{2 \log M}\right) \rightarrow 0\ ,
	%	\end{align}
	%	for any constant $\epsilon_0\in (0,1)$ and for  $\sigma_h^2 = {k \choose h} \sigma^2$.
\end{lemma}

\begin{proof}
	We apply the tail bound on the maximum of Gaussians \cite{lopes2018maximum} (\Cref{le:max-Gaussians} above) 
	with $N=C(r)=|\cN_r|$ to obtain
	\begin{align}\label{eq:max-concentration}
	\Pr\left(\max(\cN_r) \leq (1- \epsilon_0) \cdot \sigma_k  \sqrt{2 \log C(r)}\right) \rightarrow 0\ .
	\end{align}
	In particular, since in our problem the correlation vanishes, we can choose \emph{any} $\rho_0 <1$ and, for sufficiently large $n$, satisfy $\delta_0 \sqrt{1- \rho_0}\geq 1- \epsilon_0$ and $\rho(\share)\leq \rho_0$. Then, \eqref{eq:max-concentration} follows from \eqref{eq:max-Gaussians} as both $\alpha$ and $\beta$ in \eqref{eq:max-Gaussians-constants} are constants and $C(r)=|\cN_r| \rightarrow \infty$. Finally, recall that $\rate{C(r)}= \log C(r)/\log n$.    This completes the proof.
\end{proof}

%\begin{cor}\label{cor:max-concentration}
%	For $\mathcal R \equiv \log \frac{\binom{N}{k}}{{\cal D}(\share)}$ and for any constant $\epsilon_0 \in (0,1)$ the following holds: If the maximum correlation  vanishes, i.e, $\rho(\share) \rightarrow 0$, then 
%	\begin{align}\label{eq:cor-max-concentration}
%	\Pr\left(MAX(C(\share)) \leq (1- \epsilon_0) \cdot \sigma_k  \sqrt{2 \cal R}\right) \rightarrow 0
%	\end{align}
%		where $\sigma_k = \sqrt{\binom{k}{h}} \sigma$.
%\end{cor}

%\newcommand{\plant}{S_{\text{planted}}}

\begin{lemma}[concentration of planted solution]\label{le:planted-concentration}
	For any $\Delta = \Omega\left(\frac{\binom{k}{h}}{\log n}\right)$, it holds that 
	\begin{align}\label{eq:planted-concentration}
	\Pr\left(\plant > \beta_{k} +\sqrt{\Delta \cdot 2\log n} \right) \rightarrow 0 
	\end{align}
	where $\beta_k = \binom{k}{h} \beta$.
\end{lemma}

\begin{theorem} \label{th:LB-R}
	For any $\share$ such that the correlation $\rho(\share)$ vanishes  and $\rate{C(r)} =\Omega(1)$, and for any small constant $\epsilon_0 >$ we have
	\begin{align}
	\gamma < (1-\epsilon_0) \sqrt{\frac{\rate{C(r)}}{k}} && \Longrightarrow && \recover \rightarrow 0 \ . 
	\end{align}
	%where $\gamma \equiv \frac{\hat \mu}{\hat \sigma} \cdot\ \sqrt{\frac{\binom{k}{h}}{k}}$.
\end{theorem}

\begin{proof}
	We show that the condition on $\gamma$ implies that there exists a $t$ such that 
	\begin{align}\label{eq:max-and-planted-vs-t}
	\Pr\left(\max(\cN_r) > t\right) \rightarrow 1 && \text{ and } && 	\Pr\left(\plant \leq  t \right) \rightarrow 1
	\end{align}
	thus implying 
	\begin{align*}
	\recover \leq	\Pr\left(\max(\cN_r) \leq \plant \right) \leq \Pr\left(\max(\cN_r) \leq  t\right) + \Pr\left(t < \plant \right) \rightarrow 0\ . 
	\end{align*}
	To this end, as we want to apply Lemma~\ref{le:max-concentration} and Lemma~\ref{le:planted-concentration} to get \eqref{eq:max-and-planted-vs-t}, we impose that
	\begin{align*}
	(1-\varepsilon_0) \sqrt{\binom{k}{h}}  \sqrt{\rate{C(r)}\cdot 2\log n} >&  \binom{k}{h}\beta +   \sqrt{\Delta \cdot 2\log n}
	\end{align*}  
	for  $\Delta = \delta_0 \cdot  \frac{\binom{k}{h}}{\log n} $ with $\delta_0>0$ constant (we need $\Delta = \Omega\left(\frac{\binom{k}{h}}{\log n}\right)$ to apply Lemma~\ref{le:planted-concentration}). The inequality above is equivalent to the following inequalities (since $\beta = \gamma \sqrt{\frac{k}{{k \choose h}}\cdot 2 \log n}$):
	\begin{align*}
	(1-\varepsilon_0) \sqrt{\binom{k}{h}}  \sqrt{\rate{C(r)}\cdot 2\log n} >&  \sqrt{\binom{k}{h}}\gamma \sqrt{k \cdot 2\log n} +   \sqrt{2\delta_0\binom{k}{h}} \\
	(1-\varepsilon_0)   \sqrt{\rate{C(r)}} >&  \gamma \sqrt{k} +   \sqrt{\delta_0/\log n} \\
	(1-\varepsilon_0)   \sqrt{\frac{\rate{C(r)}}{k}} - \sqrt{\frac{\delta_0}{k\log n}}  >&  \gamma  
	\end{align*}
	From the hypothesis that $\rate{C(r)} =\Omega(1)$, the condition above is implied by the hypothesis $\gamma < (1-\epsilon_0) \sqrt{\frac{R(r)}{k\log n}}$, for any constant   $\varepsilon_0<\epsilon_0$ (e.g., $\varepsilon_0 = \epsilon_0/2$).
\end{proof}

Combining the  bound on $\rate{C(r)}$ in Lemma~\ref{le:R-lb} with Theorem~\ref{th:LB-R} we get \Cref{th:LB:max-Gaussians}.

\begin{proof}[Proof of \Cref{th:LB:max-Gaussians}]
	Consider any $\share = \lambda k$ with $\lambda$ being any constant satisfying \eqref{eq:linear-ell-cases}, according to the regime of $h$ vs $k$.  By  Lemma~\ref{le:vanishing-corr}, the correlation $\rho(\share)$ vanishes since $h =\omega(1)$.
	We can thus apply Theorem~\ref{th:LB-R} and Lemma~\ref{le:R-lb} with $\share = \lambda k$ and obtain the desired result as follows: 
	\[
	(1-\epsilon_0) \sqrt{\frac{\rate{C(r)}}{k}} \stackrel{(Lemma~\ref{le:R-lb})}{\geq} (1-\epsilon_0) \sqrt{\lambda(1-\alpha)} > \gamma
	\]
	where the last inequality follows from the condition on $\gamma$ in \eqref{eq:lambda-LB-cor} and the hypothesis that $\lambda$ satisfies \eqref{eq:linear-ell-cases}. The above inequality and Theorem~\ref{th:LB-R} implies the result.
	%	
	%	Since $\eta_0 <\sqrt{1/e}$, we can write $\eta_0 = \frac{1-\epsilon_0}{\sqrt{c_0}}$ for constants $\epsilon_0 \in (0,1)$ and $c_0 >e$. For $\share = k/c_0$, the correlation $\rho(\share)$ vanishes since $h = \omega(1)$ (Lemma~\ref{le:vanishing-corr}). We can thus apply Theorem~\ref{th:LB-R} and Lemma~\ref{le:R-lb} with $\share = k/c_0$ and obtain the desired result: 
	%	\[
	%	(1-\epsilon_0) \sqrt{\frac{\mathcal R}{k\log N}} \stackrel{(Lemma~\ref{le:R-lb})}{\geq} (1-\epsilon_0) \sqrt{\frac{1-\alpha}{c_0}} = \eta_0 \sqrt{1-\alpha}> \gamma
	%	\]
	%	and the above inequality $\gamma < (1-\epsilon_0) \sqrt{\frac{\mathcal R}{k\log N}}$ implies $P_{success} \rightarrow 0 $ by Theorem~\ref{th:LB-R}.
\end{proof}

%\begin{proof} Using the Vandermonde identity we have 
%	\begin{align*}
%			{\cal D}(\share) = & \sum_{d=\share}^k \binom{k}{d}\binom{N-2k}{k - d} = \sum_{d=0}^k \binom{k}{d}\binom{N-2k}{k - d} - \sum_{d=0}^{\share-1} \binom{k}{d}\binom{N-2k}{k - d} \\
%			= & \binom{N-k}{k}- \sum_{d=0}^{\share-1} \binom{k}{d}\binom{N-2k}{k - d}
%			\intertext{and since $\share \leq k\leq (N-2k)/2$ implies $\binom{N-2k}{\share-d} \leq \binom{N-2k}{k-d}$}
%			\leq  & \binom{N-k}{k}- \sum_{d=0}^{\share-1} \binom{k}{d}\binom{N-2k}{\share -1 - d}
%			\\
%			=  & \binom{N-k}{k}- \binom{N-k}{\share -1} \\
%			\approx & \binom{N}{k} - \binom{N}{\share}
%	\end{align*}
%	Since $\log (b-a) \leq \log b - \log a$ for $b>a>1$, 
%\begin{align}
%	{\cal R} =\log\frac{\binom{N}{k}}{{\cal D}(\share)} = \log\frac{\binom{N}{k}}{\binom{N}{k} - \binom{N}{\share}}\log \binom{N}{k} - \log {\cal D}(\share) \gtrsim  \log \binom{N}{k} - \log \left[\binom{N}{k} - \binom{N}{\share} \right] \geq \log \binom{N}{\share}\ . 
%\end{align}
%\end{proof}

\subsection{Proof of \Cref{th:infoTheoretic}}
\label{sec:proof:LB2}
\begin{proof} For any $x\in \CNK$, let $\bW=\bW(x)$ be the corresponding tensor according to our problem \eqref{eq:weight-def}. Consider any estimator $\hat v()$ which, for any tensor, returns some feasible solution, i.e., $\hat v(\bW)\in \CNK$. 
	%		\begin{align}
	%		\gamma \le \sqrt{\frac{1-\alpha}{2}} - \eps \;\;\Rightarrow\;\;
	%		\E\,\Loss(\hat v,x)\ge 1\,
	%		%
	%	    \end{align}
	Let $\sU(\bW)$ denote the  ${n \choose h}$-dimensional vector obtained by flattening the symmetric $h$-tensor $\bW$ into a vector containing its independent components (all $\bW_{i_1i_2\cdots i_h}$ for distinct $h$-tuples $i_1<i_2<\cdots < i_h$). Since each component  of vector $\sU(\bW)$  is a Gaussian r.v.  according to \eqref{eq:weight-def}, 
	the whole vector $\sU(\bW)$ is also distributed as 
	a Gaussian,
	\begin{align}\label{eq:flat-low}
	\sU(\bW(x)) \sim \Gaussian \left ( \beta  \sU(x^{\otimes h}) , \id_{{n \choose h}} \right )\equiv P_x \
	\end{align}
	where $\id_{{n \choose h}}$ is the identity matrix in $\reals^{n \choose h}$.
	\begin{lemma}
		\label{lem:Kullback} 
		For any two vectors $x,x' \in \CNK$ we have
		\begin{align*}
		D(P_x \Vert P_{x'}) \le \binom{k}{h}\beta^2\ ,
		\end{align*}
		where  $D(\cdot \Vert\cdot)$ denotes
		the Kullback-Leiber divergence. 
	\end{lemma}
	\begin{proof}
		Since $P_x$ and $P_{x'}$ are a Gaussian probability distributions \eqref{eq:flat-low}, we have
		\begin{align*}
		D(P_x \Vert P_{x'}) &=  \frac{1}{2} \beta^2  \|\sU(x\oh) - \sU(x'\oh)\|_2^2 \\
		&= \beta^2 ( \|\sU(x\oh) \|_2^2 
		- \<\sU(x\oh),\sU(x'\oh)\> ) 
		\\
		&\le \beta^2 \|\sU(x\oh) \|_2^2 =  \beta^2\binom{k}{h}\ .
		\end{align*}
		This completes the proof.
	\end{proof}

	For any $l\in \{0,\ldots,k\}$ and for $r=k-l$, let $\cN_r$ be the subset of solutions defined according to Lemma~\ref{le:cover}. For any  $\hat v \in \CNK$ (possibly $\hat v \not \in \cN_r$) we consider its ``closest'' vector in  $\cN_r$, 
	\[
	\G(\hat v) \equiv \argmin_{y\in\cN_r} \Loss(\hat v, y)\ .
	\] 
	By definition of $\G()$, the   event $\{\G(\hat v)\ne x\}$
	implies $\Loss(\hat v, x) \ge l/2$. By Markov inequality, for $x$ is chosen uniformly at random in $\cN_r\subseteq \CNK$,
	\begin{align}
	\prob \left(\G(\hat v(\bW)) \ne x\right) &\le \prob\left(\Loss(\hat v(\bW), x) \ge l/2\right)  \le \frac{\E~\Loss(\hat v,x)}{l/2}  
	\label{eq:Perrbound}
	\end{align}
	where $\bW=\bW(x)$
	and $\hat v()$ is any estimator. By Fano's inequality \cite{cover1999elements} we have 
	\begin{align}
	\label{eq:FanoIneq}
	\prob\left(\G(\hat v(\bW)) \ne x\right) &\ge 1-\frac{{\rm I}(x;\bW)+\log 2}{\log|\cN_r|} 
	%\ge 1 - \frac{D_{\max} + \log 2}{\log{|\cN|}}, 
	\end{align}
	where $\rm I(\cdot;\cdot)$ denotes the mutual information;  using the generalized Fano's inequality \cite{verdu1994generalizing}
	\begin{align}
	\label{eq:generalized_fano}
	{\rm I}(x;\bW) \le \frac{1}{|\cN|^2}\sum_{x\ne
		x'\in\cN}D(P_x \Vert P_{x'}) \le  \binom{k}{h} \beta^2 \ ,
	\end{align}
	where the second inequality follows from \Cref{lem:Kullback}. Hence,  since $\beta^2 = \gamma^2  \frac{k}{{k \choose h}}\cdot 2\log n$, we get
	\begin{align}
	\prob\left(\G(\hat v(\bW)) \ne x\right) &\ge 1- \frac{\binom{k}{h} \beta^2 + \log
		2}{\log|\cN|}  \approx 1- \frac{2\gamma^2 k \cdot \log n}{\log|\cN|} = 1- \frac{2\gamma^2 k}{\rate{C(r)}}
	\end{align}
	where last equality is just the definition of $\rate{C(r)}$ in \eqref{eq:rate} and the previous approximation comes from $|\cN_r|\rightarrow \infty$. 
	The bound  $\rate{C(r)} \gtrsim r(1-\alpha)$ in  Lemma~\ref{le:R-lb}, with $r = \lambda k$ and $\lambda \in (0,1)$ constant, yield
	\begin{align}\label{eq:prov-fail:tensor-proof}
	\prob\left(\G(\hat v(\bW)) \ne x\right) &\gtrsim 1- 2\gamma^2 \frac{1}{\lambda(1-\alpha)} \ .
	\end{align}
	Finally, since $l = k - r = (1-\lambda)k$
	\begin{align} 
	%\inf_{\hat v\in\cV}\sup_{x \in
	%	\CNK}
	\E~\Loss(\hat v, x) \gtrsim \frac{l}{2}\left(1- 2\gamma^2 \frac{1}{\lambda(1-\alpha)}   \right) = \frac{(1-\lambda) k}{2}\left(1- 2\gamma^2 \frac{1}{\lambda(1-\alpha)}   \right) \ ,
	\end{align}
	and the condition for impossibility of exact recovery, using a simple Markov inequality becomes $\E~\Loss(\hat v, x)\ge 1$, hence
	\begin{align} 
	\gamma \leq \sqrt{\frac{\lambda (1-\alpha) }{2} - \frac{\lambda (1-\alpha)}{(1-\lambda) k}  \lambda(1-\alpha) }.
	\end{align}
	Since this holds for any constant $\lambda \in (0,1)$ and for $k \to +\infty$ the theorem follows. 
\end{proof}

\section{Proofs for \Cref{sec:UB}}
\label{app:proofs_UB}
\begin{proof}[Proof of \Cref{le:UB-concentration}]
	Observe that each $S^{(-F)}$ consists of $d({k'}) = \binom{k}{h} - \binom{k'}{h}$ non-biased edges, and therefore $S^{(-F)} \sim \Gaussian(0,d({k'}))$. 
	Hence, by applying  \cref{eq:Gaussian} with $t= t_\Delta = \sqrt{\Delta 2\log n}$ we have 
	\begin{align}
	\label{eq:proof:single-sol-m-overlap}
	\Pr\left(S^{(-F)} > t_\Delta \right)  \stackrel{\eqref{eq:Gaussian}}{\leq} & \frac{1}{t_\Delta}\cdot \frac{e^{-t^2_\Delta/2d({k'})}}{\sqrt{2\pi}} 
	=
	\frac{e^{-(\Delta \log n)/d({k'})}}{t_\Delta \sqrt{2\pi}}  
	= 
	\frac{n^{-\Delta/d({k'})}}{\sqrt{2\pi \Delta} \cdot \sqrt{2 \log n}}  \ ,
	\end{align}
	which proves \cref{eq:bound-generic:m-intersecting}. By the union bound and \cref{eq:bound-generic:m-intersecting} we obtain \cref{eq:LB-bound:m-intersecting}:
	\begin{align*}
	\Pr\left(\max(\S_{k'}^{(-F)}) >t\right) =& \Pr\left(\bigcup_{S^{(-F)} \in \S_{k'}^{(-F)}} S>t\right)   \leq Q_{k'} \cdot p_{{k'},\Delta}\ . 
	\end{align*}
	Finally, \cref{eq:UB-bound:planted} holds by observing that, since all $d({k'})$ edges of $\plant^{(-F)}$ are biased, we have  $\plant^{(-F)}\sim \Gaussian(d({k'})\beta,d({k'}))$. Therefore, by applying \cref{eq:Gaussian} with $t= d({k'})\beta + t_\Delta$ we get
	\begin{align*}
	\Pr\left(\plant^{(-F)}< d({k'})\beta -t_\Delta\right) &= \Pr\left(\plant^{(-F)}> d({k'})\beta +t_\Delta\right)  \stackrel{\eqref{eq:Gaussian}}{\leq} \frac{1}{t_\Delta}\cdot \frac{e^{-t^2_\Delta/2d({k'})}}{\sqrt{2\pi}} \end{align*} and the remaining of the proof is as above in \cref{eq:proof:single-sol-m-overlap}. 
\end{proof}

\begin{proof}[Proof of \Cref{th:UB-with-eta}]
	For any ${k'}\in \{0,\ldots k-1\}$ we have 
	\begin{align}
	\label{eq:simple_UB}
	\Pr\left(\max(\S_{k'}) >  \plant\right) &\leq \binom{k}{{k'}} \Pr\left(\max(\S_{k'}^{(F)})> \plant\right) \nonumber \\
	&=\binom{k}{{k'}} \Pr\left(\max(\S_{k'}^{(-F)})> \plant^{(-F)}\right)
	\end{align}
	We show below that $\gamma > \gamma^{({k'})}_{UB_\eta}$ implies that there exists $t$ such that
	\begin{equation}
	\label{eq:threshold:separation}
	t_{\Delta'} < t < d({k'}) \beta - t_{\Delta''}
	\end{equation}
	with
	\begin{equation}
	\label{eq:UB:separation}
	\frac{\Delta'}{d({k'})} \geq   \frac{\log M_{k'}}{\log N} + \eta\ \quad \text{and} \quad \frac{\Delta''}{d({k'})} \geq \frac{\log {k \choose {k'}}}{\log n} + \eta \ .
	\end{equation}
	Since $\Pr(X>Y) \leq \Pr(X>t) + \Pr(t \geq Y)$ for every $t$, we have  
	\begin{align}
	\label{eq:simple_UB_two_terms}
	\Pr\left(\max(\S_{k'}^{(-F)})>\plant^{(-F)}\right) &\leq \Pr\left(\max(\S_{k'}^{(-F)})>t\right) \nonumber +\Pr\left(t\geq  \plant^{(-F)}\right) \nonumber \\ 
	&\leq \Pr\left(\max(\S_{k'}^{(-F)})>t_{\Delta'}\right) +\Pr\left(d({k'})\beta-t_{\Delta''}>\plant^{(-F)}\right) \nonumber \\
	&\leq Q_m \cdot p_{{k'},\Delta'}+p_{{k'},\Delta''}
	\end{align}
	where the latter inequality follows from  \cref{eq:UB-bound:planted} and \cref{eq:LB-bound:m-intersecting}. 
	Combining \cref{eq:simple_UB} and \cref{eq:simple_UB_two_terms}, we get 
	\begin{align*}
	\Pr(\max(\S_{k'})> \plant)   
	\leq 
	\binom{k}{k'} (Q_m \cdot p_{{k'},\Delta'} + p_{{k'},\Delta''})   
	& =  \\ \binom{k}{k'}\left(\left(\frac{1}{n}\right)^{\frac{\Delta'}{d({k'})}} \frac{Q_m}{\sqrt{2\pi \Delta'} \cdot \sqrt{2 \log n}} \right) +\binom{k}{k'}\left( \left(\frac{1}{n}\right)^{\frac{\Delta''}{d({k'})}} \frac{1}{\sqrt{2\pi \Delta''} \cdot \sqrt{2 \log n}}\right)
	&=\\
	\left(\left(\frac{1}{n}\right)^{\frac{\Delta'}{d({k'})} - \frac{\log M_{k'}}{\log n}} \frac{1}{\sqrt{2\pi \Delta'} \cdot \sqrt{2 \log n}} \right)
	+\left(  \left(\frac{1}{n}\right)^{\frac{\Delta''}{d({k'})}- \frac{\log \binom{k}{k'}}{\log n}} \frac{1}{\sqrt{2\pi \Delta''} \cdot \sqrt{2 \log n}}\right)
	\end{align*}
	where we used in the first equality \cref{eq:bound-generic:m-intersecting} and in the last equality the identity $z = n^{\frac{\log z}{\log n}}$ and the fact that ${k \choose h } Q_{k'} = \binom{k}{h} \binom{n - k}{k-k'}= M_{k'}$. Then, by \cref{eq:UB:separation} we get the next two inequalities
	\begin{align*}
	\Pr(\max(\S_{k'}) >\plant)  &\leq \frac{1}{n^\eta} \frac{1}{\sqrt{2\pi} \cdot \sqrt{2 \log n}}\left(\frac{1}{\Delta'}+ \frac{1}{\Delta''}\right)  
	\\&\leq  \frac{1}{n^\eta} \frac{1}{\sqrt{2\pi} \sqrt{2\log n} \cdot d({k'})} \left(\frac{\log n}{\log M_{k'}}+\frac{\log n}{\log {k \choose {k'}}}\right) \\
	&\leq \frac{1}{n^\eta} \frac{\sqrt{\log n}}{\sqrt{\pi}}
	%&\leq \frac{1}{N^\eta} \frac{2}{\sqrt{2\pi} \cdot \hat \sigma \cdot \log k}
	\end{align*}
	where in the last inequality we used $d({k'}) \geq 1$, for ${k'} \in \{0,\ldots, k-1\}$, and $M_{k'} \geq {k \choose h} \geq k$. 
	
	To conclude the proof we show that $\gamma > \gamma^{({k'})}_{UB_\eta}$ implies that  there exists $t$ such that \cref{eq:threshold:separation} and \cref{eq:UB:separation} hold. We set $\Delta' =   d({k'})\left(\frac{\log M_{k'}}{\log n} + \eta\right)$   and  $\Delta'' = d({k'}) \left(\frac{\log {k \choose {k'}}}{\log n} + \eta \right)$ so that \cref{eq:UB:separation} holds. 
	%Then we observe that $\frac{\log M_{k'}}{\log N} \approx (k-k')(1+\beta_0-\beta_0'$) and $\frac{\log {k \choose {k'}}}{\log N}  \approx (k-k')(\beta_0 -\beta_0')$. Hence, $\Delta' \approx d({k'})[ (k-k')(1+\beta_0-2\beta_0')+ \eta]$ and $\Delta'' \approx d({k'}) [(k-k')(\beta_0-\beta_0') + \eta]$. 
	By plugging this into \cref{eq:threshold:separation}, we can rewrite the inequality $t_{\Delta'}  < d({k'}) \beta - t_{\Delta''}$ as follows:
	\begin{align*}
	d({k'}) \beta &>  t_{\Delta'} + t_{\Delta''}  \stackrel{\eqref{eq:threshold-plus-min}}{>} \sqrt{2 \log n}(\sqrt{\Delta'} + \sqrt{\Delta''})  
	\end{align*}
	hence by the rescaling in \cref{eq:rescaling} we get the condition for the SNR:
	\begin{align*}
	\frac{\beta}{\sqrt{2 \log n}} &>  \frac{1}{d({k'})}(\sqrt{\Delta'} + \sqrt{\Delta''}) \\
	&=\sqrt{\frac{1}{d({k'})}} \left(\sqrt{\frac{\log M_{k'}}{\log n}+\eta}  + \sqrt{\frac{\log { k \choose {k'}}}{\log n}+\eta}\right) \\
	&= \sqrt{\frac{1}{d(k')}} \cdot UB_{\eta}({k'})
	\end{align*}
	and the theorem follows from the identity definition of $\gamma$ in \cref{eq:rescaling}.
\end{proof}
\begin{proof}[Proof of \Cref{th:UB}]
	We first show the following result:
	\begin{lemma}\label{le:gamma-constants}
		For every $k$ and $k'\in\{0,\ldots,k-1\}$, it holds that
			\begin{align}
			\gamma^{({k'})}_{UB_\eta}  \leq & \left(\sqrt{1+ \rate{k}-2 \rate{k}'+\eta} + \sqrt{\rate{k} - \rate{k}'+\eta}\right)\sqrt{\frac{(k-{k'})\binom{k}{h}}{(\binom{k}{h} - \binom{k'}{h}) k }}
			\label{eq:lemma_first_part}\\ 
			\leq &  \left(\sqrt{1+ \rate{k}-2 \rate{k}'+\eta} + \sqrt{\rate{k} - \rate{k}'+\eta}\right) \ .
			\end{align}
%		\begin{align}
%		\gamma^{({k'})}_{UB_\eta}  \leq & \left(\sqrt{1+ \beta_0-2 \beta_0'+\eta} + \sqrt{\beta_0 - \beta_0'+\eta}\right)\sqrt{\frac{k-{k'}}{\binom{k}{h} - \binom{k'}{h}}} 
%		\label{eq:lemma_first_part}\\ 
%		\leq &  \left(\sqrt{1+ \beta_0-2 \beta_0'+\eta} + \sqrt{\beta_0 - \beta_0'+\eta}\right)\sqrt{\frac{k}{\binom{k}{h}}} \ .
%		\end{align}
	\end{lemma}
	
	\begin{proof}[Proof of Lemma~\ref{le:gamma-constants}]
%		Note  that
%		\[
%		{k \choose {k'}} = {k \choose k-{k'}} \leq e^{k-{k'}} \left(\frac{k}{k-{k'}}\right)^{k-{k'}} \ .
%		\]
%		thus implying 
%		
		Using the standard inequalities on binomial coefficients in \cref{eq:log-bonimial} we have
		\begin{align*}
		\frac{\log {k \choose {k'}}}{\log n} \leq &  (k-{k'})\frac{1 + \log k - \log (k-{k'})}{\log n}  \stackrel{\eqref{eq:rate}}{\approx}  (k-{k'}) (\rate{k} - \rate{k - k'})  \ ,
		\\
		\frac{\log {n-k \choose k -{k'}}}{\log n} \leq &  (k-{k'})\frac{1 + \log (n-k) - \log (k-{k'})}{\log n}    \stackrel{\eqref{eq:rate}}{\approx}   (k-{k'}) (1 - \rate{k - k'})  \ ,\\ 
		\end{align*}
		thus implying 
		\begin{align*}
		\frac{\log M_{k'}}{\log n} = \frac{\log \left({k \choose {k'}}{n-k \choose k-{k'}}\right)}{\log n} & \lesssim (k-{k'})(1+ \rate{k} -2 \rate{k - k'}) \ .
		\end{align*}
		By plugging this into the definition of $UB_\eta({k'})$ in \cref{eq:UB:gamma-k}, we get
		\begin{align*}
		UB_\eta({k'}) = &   \sqrt{{\frac{\log M_{k'}}{\log n}}+\eta} + \sqrt{{\frac{\log  {k \choose {k'}}}{\log n}}+\eta} \lesssim  
		\sqrt{1+ \rate{k} -2 \rate{k-k'} +\eta} + \sqrt{\rate{k}  - \rate{k - k'}+\eta} \ .
		\end{align*}
		Hence, using the definition of $\gamma^{({k'})}_{UB_\eta}$ given in \Cref{th:UB-with-eta}, we obtain \cref{eq:lemma_first_part}.
		To conclude the proof we show that 
		\begin{align*}
		\frac{k-{k'}}{{k \choose h} - {{k'} \choose h}} \leq \frac{k}{{k \choose h}}\ . 
		\end{align*}
		Simply observe that this inequality is equivalent to 
		\begin{align}
		\frac{k-{k'}}{k} \leq \frac{{k \choose h} - {{k'} \choose h}}{{k \choose h}} \Leftrightarrow \frac{{{k'} \choose h}}{{k \choose h}}  \leq \frac{{k'}}{k}\ . 
		\end{align}
		For ${k'}<h$ this inequality is trivially satisfied since ${{k'} \choose h} =0$. Otherwise we can write the previous inequality as 
		\begin{align*}
		\frac{{{k'} \choose h}}{{k \choose h}} &= \frac{{k'}!}{h!({k'}-h)!}\frac{h!(k-h)!}{k!} 
		=\frac{{k'}({k'}-1)\cdots ({k'}-h+1)}{k(k-1)\cdots (k-h+1)} \leq \frac{{k'}}{k}
		\end{align*}
		which is satisfied for any ${k'} \leq k$ since all these terms satisfy $\frac{{k'}-i}{k-i} \leq 1$, for $1\leq i \leq h-1$.
	\end{proof}
	
	\paragraph*{Proof of \Cref{th:UB}}
	The idea is that by taking $\eta=\rate{k'} + \epsilon_0$, we can apply the union bound over all $m\leq k'$ to get the right hand side of \cref{eq:UB:max-based} going to  $0$, hence $\fail^{(k')} \rightarrow 0$ and $\recover^{(k')} \rightarrow 1$.  Specifically, for $\gamma$ satisfying $\gamma>\gamma^{({m})}_{UB_\eta}$ for all $m=\{0,\ldots, k'\}$, we have $\Pr\left(\max(\S_{m}) >  \plant\right) \in O\left(\frac{\sqrt{\log n}}{n^{\eta}} \right)$ thus implying
	\[
	\fail^{(k')} \in  O\left(\frac{k'\sqrt{\log n}}{n^{\eta}} \right)\ .
	\]
	For $\eta = \rate{k'}+\epsilon_0$ we have 
	\[
	\frac{k'\sqrt{\log n}}{n^\eta} = \frac{k'}{n^{\rate{k'}}} \cdot \frac{\sqrt{\log n}}{n^{\epsilon_0}} \approx  \frac{\sqrt{\log n}}{n^{\epsilon_0}}
	\]
	where the asymptotics is due to $\frac{k'}{n^{\rate{k'}}} \rightarrow 1$, by  definition of $\rate{k'}$ in \cref{eq:rate}. 
 Hence, $\frac{k'}{n^\eta} = o(1)$ and the probability $\fail^{(k')}$ tend to $0$.
\end{proof}
